# Supplementary material for: PickScan: Object discovery and reconstruction from handheld interactions
Source: arXiv:2411.11196 source file (2024-11-17)
Supplement: Supplementary file 1 [file 01-contrib.tex]

\section{Contribution statement}

\textbf{Nikhil Keetha} conceived the idea and led the project. Responsible for initial code development, writing major sections of the paper, and producing figures, tables \& videos.

\textbf{Avneesh Mishra} implemented vital components, including the foundation model feature extraction and modular scripts, to run experiments at a large scale. Responsible for running the ablation experiments, writing the first draft of the results section, and producing qualitative visualizations \& the Hugging Face demo.

\textbf{Jay Karhade} scaled the evaluation to a diverse suite of unstructured environments, implemented the vocabulary ablations, and performed explorations into various foundation models, including SAM. Responsible for the website, retrieval visualizations, and diverse suite of interactive demos.

\textbf{Krishna Murthy} was actively involved in brainstorming and critical review throughout the project. Responsible for the exploration of self-supervised visual foundation models. Wrote \& proofread sections of the paper.

\textbf{Sebastian Scherer} pushed us towards evaluating the practicality of current VPR systems in unstructured environments and developing a universal VPR system. Suggested a vital paper restructuring to ensure the critical message and insights are easily parsable. Sebastian provided compute resources for initial explorations and ablations.

\textbf{Madhava Krishna} was involved in initial brainstorming discussions and provided feedback throughout the development. Suggested revisions for sections of the paper. Madhav also provided most of the compute for the experiments conducted in this work.

\textbf{Sourav Garg} provided resourceful visual place recognition perspectives and critical thoughts in the brainstorming sessions, which led to clear insights into the applicability of foundation model features for VPR. Wrote and proofread sections of the paper.
