# Supplementary material for: PickScan: Object discovery and reconstruction from handheld interactions
Source: arXiv:2411.11196 source file (2024-11-17)
Supplement: Supplementary file 2 [file 02-datasets.tex]

\section{Dataset Details}

In this section, we provide detailed descriptions of the 12 diverse datasets used for evaluation.

\subsection{Structured Environments}
\label{sec:appendix_structured}

\paragraph{Baidu Mall} This visual localization dataset consists of images captured within a mall with varying camera poses. The dataset provides groundtruth location and 3D pose of an image, making it suited for both 6-Degrees of Freedom (DoF) Localization and VPR testing. We use the entire dataset consisting of $2292$ query images \& $689$ reference images for evaluation. This mall dataset presents interesting and challenging properties, including perceptually aliased structures, distractors for VPR (such as people), and semantically rich information, such as billboards and signs.

\paragraph{Gardens Point} This dataset contains two traverses through the Gardens Point campus of Queensland University of Technology (QUT) captured at different times of the day, i.e., day and night. Both the database and query traverses contain $200$ images, respectively. The drastic lighting changes and transitions from indoor to outdoor scenarios make it a difficult VPR dataset.

\paragraph{17 Places} This indoor dataset consists of traverse collected within buildings at York University (Canada) and Coast Capri Hotel (British Columbia). The reference and query traverses consist of $406$ images. The high clutter, change in lighting conditions, and semantically rich information make this dataset interesting.

\paragraph{Pittsburgh-30k} This benchmark VPR dataset consists of images collected at various locations and poses throughout downtown Pittsburgh. We use the test split consisting of $10,000$ database images and $6816$ query images. This dataset is challenging due to the presence of drastic viewpoint shifts, a large variety of geometric structures such as buildings, and distractors such as cars and pedestrians.

\paragraph{St Lucia} This dataset consists of daytime traverses collected using a stereo camera pair on a car, where the traverses span a total distance of $9.5$ km. The reference traverse consists of $1549$ images, while the query traverse consists of $1464$ images. A large number of loop closure events, reverse traverses, shadows, and vegetation make this dataset challenging.

\paragraph{Oxford RobotCar} This dataset consists of Oxford City traverses, which showcase shifts in seasonal cycles and daylight. We use a subsampled version of the Overcast Summer and Autumn Night traverses, similar to HEAPUtil~\cite{keetha2021hierarchical}. The original traverses are subsampled with an approximate spacing of $5$ meters to obtain a total of $213$ frames in the summer traverse and $251$ frames in the autumn night traverse with a total distance spanning $1.5$ Km. This dataset presents a challenging shift in visual appearance caused by the time of day and seasonal shifts.

\subsection{Unstructured Environments}
\label{sec:appendix_unstructured}

\paragraph{Hawkins} This dataset is an indoor mapping of an abandoned multi-floor hospital in Pittsburgh, where it is particularly challenging due to long corridors with visually-degraded features~\cite{zhao2023subtmrs}. 
In particular, we use a long corridor spanning $282$ m with a localization radius of 8 m, where the database and query images are collected from 2 opposing viewpoints (forward \& backward direction). 
The database and query set contain $65$ and $101$ images, respectively.

\paragraph{Laurel Caverns} This subterranean dataset consists of images collected using a handheld payload~\cite{zhao2023subtmrs}. 
The low illumination scenarios and lack of rich visual features make this dataset particularly challenging. 
The opposing viewpoint of the database and query images adds additional complexity to the strong distribution shift.
We use a $102$ m trajectory with a localization radius of 8 m, where the database and query sets contain $141$ and $112$ images, respectively.

\paragraph{Nardo-Air} This is a GNSS-denied localization dataset collected using a $100^{\circ}$ FoV downward-facing camera on board a hexacopter flying at $10$ m/s and an altitude of $50$ m across a grass-strip runway named Nardo. The reference database comprises $102$ images obtained from a Google Maps TIF satellite image, while the query set contains $71$ drone-collected imagery. The perceptual aliasing at the end of the runway and non-typical vegetative features combined with a long time shift make this dataset challenging. The -R variant of this dataset indicates rotation where the drone imagery is rotated to match the satellite image orientation. We use a $700$ m trajectory spanning across a square kilometer area, where the localization radius is $60$ m.

\paragraph{VP-Air} This aerial VPR dataset consists of $2,706$ database-query image pairs and $10,000$ distractors collected at $300$ m altitude with a downward-facing camera on an aircraft~\cite{schleiss2022vpair}. The dataset spans over $100$ km, encompassing various challenging landscapes such as urban regions, farmlands, and forests. We use a localization radius of $3$ frames.

\paragraph{Mid-Atlantic Ridge} We construct this dataset using the overlapping sequences of an underwater visual localization dataset~\cite{boittiaux2022eiffel}. It presents OOD challenges including seabed objects, low illumination, and appearance shifts over a long time period (2015 vs. 2020). The dataset contains $65$ database images and $101$ query images, where the trajectory spans $18$ m and the localization radius is $0.3$ m.
