# Supplementary material for: PickScan: Object discovery and reconstruction from handheld interactions
Source: arXiv:2411.11196 source file (2024-11-17)
Supplement: Supplementary file 3 [file 03-content.tex]

% \begin{figure*}[!t]
% \centering
% \begin{tabular}{cccc}
% \includegraphics[width=0.225\linewidth]{figures/ablations/layer/DINOv2_ViT_S14.pdf} 
% &
% \includegraphics[width=0.225\linewidth]{figures/ablations/layer/DINOv2_ViT_B14.pdf} 
% &
% \includegraphics[width=0.225\linewidth]{figures/ablations/layer/DINOv2_ViT_L14.pdf} 
% &
% \includegraphics[width=0.225\linewidth]{figures/ablations/layer/DINOv2_ViT_G14.pdf} 
% \end{tabular}
% \caption{\textbf{Ablation across \coolagg{\dinovtwo}{VLAD} ViT Model Size}: Recall@1 across different DINOv2 ViTs \& feature layers on the Baidu Mall and Oxford RobotCar datasets. Performance scales with the model size but saturates at ViT-L. Across the different ViT model sizes, performance peaks at intermediate layers instead of the final layer.}
% \label{fig:layer_ablation}
% \end{figure*}

% \section{AnyLoc: ViT Ablations}

% \begin{figure}[!t]
% \centering
% \begin{tabular}{cccc}
% \includegraphics[width=0.45\linewidth]{figures/ablations/layer/DINO_ViT_S8_Key.pdf} 
% &
% \includegraphics[width=0.45\linewidth]{figures/ablations/layer/DINO_ViT_S8_Value.pdf} 
% \end{tabular}
% \caption{Ablation study comparing the Recall@1 of the Key and Value facet features across different DINO ViT-S8 layers on the Baidu Mall and Oxford RobotCar datasets.}
% \label{fig:layer_ablation_dino}
% \end{figure}

% \begin{figure}[!t]
% \centering
% \begin{tabular}{cccc}
% \includegraphics[width=0.45\linewidth]{figures/ablations/facet/DINO_ViT_S8_L9.pdf} 
% &
% \includegraphics[width=0.45\linewidth]{figures/ablations/facet/DINOv2_ViT_G14.pdf} 
% \end{tabular}
% \caption{Ablation study comparing the Recall@1 across different DINO \& DINOv2 facets on the Baidu Mall and Oxford RobotCar datasets.}
% \label{fig:facet_ablation}
% \end{figure}
