# Supplementary material for: PickScan: Object discovery and reconstruction from handheld interactions
Source: arXiv:2411.11196 source file (2024-11-17)
Supplement: Supplementary file 4 [file 04-related.tex]

% \subsection{Self-Supervised learning for VPR}

% Beyond the widely used contrastive learning-based weak supervision, few self-supervised approaches have been proposed for learning visual representations in the context of place recognition. 
% One such approach explores the use of synchronization across multiple sensors to learn a distance metric for arbitrary image descriptors, enabling self-supervised VPR learning in mobile robots~\cite{pillai2019self}. 
% TF-VPR~\cite{chen2022self} proposes using temporal and feature neighborhoods to discover unknown spatial neighborhoods. 
% This, coupled with a positive set contraction based on geometric verification, allows TF-VPR to train learning-based models for VPR in a self-supervised manner. 
% More recently, a self-supervised domain calibration approach for VPR has been proposed to deal with the out-of-distribution generalization issues caused by learning-based methods~\cite{lajoie2022self}. 
% In particular, a robust pose graph optimization is used to finetune the network online on the target environment without requiring any GPS or manual labeling. 
% While these approaches provide promising directions for self-supervised adaptation in the context of VPR, our zero-shot VPR approach leverages the open-set properties of foundation models to achieve robust performance in diverse scenarios without requiring finetuning.

% \subsection{Foundation Models}

% Intro to Foundation Models (Not very Relevant)
% Recent advances in deep learning are a consequence of training models with billions of parameters over web-scale data comprising images, text, audio, and other modalities.
% These models (coined \emph{foundation models}~\cite{fmodels}), e.g., CLIP~\cite{radford2021learning}, \dino{}~\cite{caron2021emerging}, \dinovtwo{}~\cite{oquab2023dinov2}, and SAM~\cite{kirillov2023segment}, have been demonstrated to learn general-purpose feature representations that work out-of-the-box (i.e., zero-shot) on a number of downstream tasks.
% , and are inherently open-set (i.e., not restricted to a set of training categories).
% Models such as are successful examples of this paradigm.
% In the robotics research community, foundation models are already being leveraged to build generalist agents that are capable of performing a diverse set of downstream tasks without requiring task-specific training~\cite{rt12022arxiv, jatavallabhula2023conceptfusion, kumar2022pre, shah2023vint, li2022language}.
% However, their applicability to building a general-purpose VPR solution that works across environments, remains unexplored.
% large-scale, multi-modal models (coined ``Foundation Models") that are trained on vast amounts of data consisting of images, text, audio, and various other modalities~\cite{fmodels}. 
% Examples of such models include CLIP~\cite{radford2021learning}, \dino{}~\cite{caron2021emerging}, \dinovtwo{}~\cite{oquab2023dinov2}, AudioCLIP~\cite{audioclip}, Segment Anything Model (SAM)~\cite{kirillov2023segment}, and their variations, which have exhibited impressive performance on open-set scenarios.  In the same spirit, foundation models are being leveraged in robotics research to create generalist agents capable of performing multiple downstream tasks in a zero- or few-shot manner~\cite{rt12022arxiv,jatavallabhula2023conceptfusion,kumar2022pre,shah2023vint}. More recent work has also shown that zero-shot adaptation is preferable over task-specific training or finetuning~\cite{li2022language} to avoid forgetting~\cite{ding2022don,jatavallabhula2023conceptfusion}, which can limit the open-set reasoning required by robotic perception systems for tasks like localization and navigation.
% Given this meteoric rise of Foundation Models, numerous approaches have been proposed to finetune these models for downstream tasks. 
% Such approaches tend to ground the foundation models to the downstream task or align image-level features to 2D pixels~\cite{li2022language}. 
% The invariance and semantic properties of the underlying features of these models have been studied at pixel- and object-level ~\cite{park2023self, shekhar2023objectives, jatavallabhula2023conceptfusion}, resulting in their successful use even in the fine-grained task of dense feature correspondence~\cite{amir2021deep}. However, the utility of these features to form robust global image representations still remains unexplored, particularly in the context of `place'-type imagery, where recent work in this direction is only limited to small-scale indoor experiments or vision-language use-cases~\cite{radford2021learning,mirjalili2023fm, kassab2023clip}.   
% One such work explored the properties of \dino{}~\cite{caron2021emerging} (a self-supervised Vision Transformer (ViT)) for dense visual descriptor extraction~\cite{amir2021deep}.
% It was showcased that these self-supervised ViT features encode rich semantic information across object categories with fine granularity, allowing them to be used as zero-shot dense visual descriptors for various applications, including part co-segmentation and keypoint correspondence.

% Recently, in the context of visual localization, few approaches have explored the semantic properties of CLIP~\cite{radford2021learning} features to perform indoor localization~\cite{mirjalili2023fm, kassab2023clip}. 
% One such approach, FM-Loc~\cite{mirjalili2023fm}, leverages the visual-language grounding offered by CLIP and GPT-3 to detect objects and room labels of a query image and uses that semantic information to match it with reference images. 
% On the other hand, another approach explores the naive use of the CLIP CLS token as an image descriptor for VPR, showcasing competitive performance compared to NetVLAD on indoor datasets~\cite{kassab2023clip}. 
% Although these approaches display the potential of visual-language features for indoor VPR, they don't explore the broad applicability of foundation model features in the context of ``places" and the use of classical aggregation techniques to achieve zero-shot VPR on a diverse range of domains.
